# Supplementary material for: The direct correlation function of a crystalline solid
Source: arXiv:2104.11558 ancillary file (2021-04-26)
Supplement: Supplementary file 1 [file SI.pdf]

# Supplementary information of
# *The direct correlation function of a crystalline solid*


S.-C. Lin* and M. Oettel
*Institut für Angewandte Physik, Universität Tübingen, Auf der Morgenstelle 10, 72076 Tübingen, Germany*

J. M. Hring, R. Haussmann, and M. Fuchs
*Fachbereich fr Physik, Universitt Konstanz, 78457 Konstanz, Germany*

G. Kahl
*Institut fr Theoretische Physik, TU Wien, 1040 Vienna, Austria*


(Dated: April 26, 2021)


## I. WHITE BEAR II TENSORIAL FUNCTIONAL

For an introduction to Fundamental Measure Theory (FMT) we refer the reader to Ref. [1]. Here we only provide the necessary definitions for the particular functional we have used, the White Bear II tensorial functional. The free energy density $\Phi$ of the White Bear II tensorial functional is:

$$\Phi(n_\alpha) = -n_0 \ln(1-n_3) + g_2(n_3)\frac{n_1 n_2 - \mathbf{n}_1\cdot\mathbf{n}_2}{1-n_3} + g_3(n_3)\frac{n_2^3 - 3n_2\mathbf{n}_2\cdot\mathbf{n}_2 + \frac{9}{2}(\mathbf{n}_2^t\cdot\mathbf{n}_\mathrm{T}\cdot\mathbf{n}_2 - \mathrm{Tr}(\mathbf{n}_\mathrm{T}^3))}{24\pi(1-n_3)^2}, \tag{1}$$

with

$$g_2(n_3) = -\frac{(-5+n_3)n_3 + 2(-1+n_3)\ln(1-n_3)}{3n_3}$$
$$g_3(n_3) = -\frac{2\left(n_3(1+(-3+n_3)n_3) + (-1+n_3)^2\ln(1-n_3)\right)}{3n_3^2}. \tag{2}$$

The weighted densities are convolutions of the density profile $\rho(\mathbf{r})$ with weight functions, $n_\alpha(\mathbf{r}) = \int d\mathbf{r}'\,\rho(\mathbf{r}')\omega_\alpha(\mathbf{r}-\mathbf{r}')$, with the weight functions given by

$$\begin{aligned}
\omega_3(\mathbf{r}) &= \Theta(R-|\mathbf{r}|),\\
\omega_2(\mathbf{r}) &= \delta(R-|\mathbf{r}|),\\
\omega_1(\mathbf{r}) &= \frac{\omega_2(\mathbf{r})}{4\pi R},\\
\omega_0(\mathbf{r}) &= \frac{\omega_2(\mathbf{r})}{4\pi R^2},\\
\boldsymbol{\omega}_2(\mathbf{r}) &= \frac{\mathbf{r}}{|\mathbf{r}|}\delta(R-|\mathbf{r}|),\\
\boldsymbol{\omega}_1(\mathbf{r}) &= \frac{\boldsymbol{\omega}_2(\mathbf{r})}{4\pi R},\\
\boldsymbol{\omega}_\mathrm{T}(\mathbf{r}) &= \left(\frac{\mathbf{r}\,\mathbf{r}^t}{|\mathbf{r}|^2} - \frac{\mathbb{I}}{3}\right)\delta(R-|\mathbf{r}|),
\end{aligned} \tag{3}$$

where $\delta$ is the Dirac delta function, $\Theta$ is the Heaviside step function and $R=\sigma/2$ is the radius of hard spheres. The tensor weight $\boldsymbol{\omega}_\mathrm{T}$ is formed by the dyadic product $\mathbf{r}\,\mathbf{r}^t$ (where $\mathbf{r}^t$ denotes the transpose of $\mathbf{r}$) and the unit matrix $\mathbb{I}$. The Fourier transforms of the weight functions are:

$$\begin{aligned}
\widetilde{\omega}_3(\mathbf{k}) &= \frac{4\pi}{|\mathbf{k}|^3}\left(\sin(|\mathbf{k}|R) - |\mathbf{k}|R\cos(|\mathbf{k}|R)\right),\\
\widetilde{\omega}_2(\mathbf{k}) &= \frac{4\pi}{|\mathbf{k}|}R\sin(|\mathbf{k}|R),\\
\widetilde{\boldsymbol{\omega}}_2(\mathbf{k}) &= -\mathrm{i}\mathbf{k}\widetilde{\omega}_3(\mathbf{k}),\\
\widetilde{\boldsymbol{\omega}}_\mathrm{T}(\mathbf{k}) &= \left(\widetilde{\omega}_2(\mathbf{k}) - \frac{3}{R}\widetilde{\omega}_3(\mathbf{k})\right)\left(\frac{\mathbf{k}\,\mathbf{k}^t}{|\mathbf{k}|^2} - \frac{\mathbb{I}}{3}\right)
\end{aligned} \tag{4}$$

An explicit derivation of these Fourier transforms can be found in Refs. [2, 3].

## II. NUMERICAL PROCEDURE FOR THE DIRECT CORRELATION FUNCTION

The crystal direct correlation function (DCF) in FMT is (Eq. (4) in the main text):

$$\begin{aligned}
c^{\mathrm{cr}}(\mathbf{r}_1,\mathbf{r}_2) &= -\frac{\delta^2\mathcal{F}^{\mathrm{ex}}[n(\rho)]}{\delta\rho(\mathbf{r}_1)\delta\rho(\mathbf{r}_2)}\\
&= -\int\sum_{\alpha\beta}\Phi_{\alpha\beta}(\mathbf{r})\omega_\alpha(\mathbf{r}-\mathbf{r}_1)\omega_\beta(\mathbf{r}-\mathbf{r}_2)d\,\mathbf{r}
\end{aligned} \tag{5}$$

with $\Phi$ the free energy density (Eq. (1)), $\Phi_{\alpha\beta} = \frac{\partial^2}{\partial n_\alpha \partial n_\beta}\Phi$, $n$ denotes collectively the weighted densities and $\omega_\alpha$ are the weight functions of Eq. (3). Since the $\omega_\alpha$ are sharp functions in real space but have smooth analytic forms in Fourier space, it is more convenient to solve Eq. (5) in Fourier space. For the Fourier transformed DCF one


* shang-chun-lin@uni-tuebingen.de

finds

$$\tilde{c}^{\rm cr}(\mathbf{k}_1,\mathbf{k}_2) = -\iiint \sum_{\alpha\beta} \Phi_{\alpha\beta}(\mathbf{r})\omega_\alpha(\mathbf{r}-\mathbf{r}_1)\omega_\beta(\mathbf{r}-\mathbf{r}_2) \times e^{-\mathrm{i}\mathbf{k}_1\cdot\mathbf{r}_1} e^{-\mathrm{i}\mathbf{k}_2\cdot\mathbf{r}_2} d\mathbf{r}d\mathbf{r}_1 d\mathbf{r}_2$$
$$= -\iiint e^{-\mathrm{i}(\mathbf{k}_1+\mathbf{k}_2)\cdot\mathbf{r}} e^{\mathrm{i}\mathbf{k}_1\cdot(\mathbf{r}-\mathbf{r}_1)} e^{\mathrm{i}\mathbf{k}_2\cdot(\mathbf{r}-\mathbf{r}_2)} \times \sum_{\alpha\beta} \Phi_{\alpha\beta}(\mathbf{r})\omega_\alpha(\mathbf{r}-\mathbf{r}_1)\omega_\beta(\mathbf{r}-\mathbf{r}_2) d\mathbf{r}d\mathbf{r}_1 d\mathbf{r}_2$$
$$= -\sum_{\alpha\beta} \tilde{\Phi}_{\alpha\beta}(\mathbf{k}_1+\mathbf{k}_2)\tilde{\omega}_\alpha(-\mathbf{k}_1)\tilde{\omega}_\beta(-\mathbf{k}_2), \quad (6)$$

and thus the crystal DCF in real space is

$$c^{\rm cr}(\mathbf{r}_1,\mathbf{r}_2) = -\frac{1}{(2\pi)^6}\int e^{\mathrm{i}\mathbf{k}_2\cdot\mathbf{r}_2} d\mathbf{k}_2 \times \int \sum_{\alpha\beta} \tilde{\Phi}_{\alpha\beta}(\mathbf{k}_1+\mathbf{k}_2)\tilde{\omega}_\alpha(-\mathbf{k}_1)\tilde{\omega}_\beta(-\mathbf{k}_2) e^{\mathrm{i}\mathbf{k}_1\cdot\mathbf{r}_1} d\mathbf{k}_1 \quad (7)$$

Calculating the DCF in this form is referred to as the "brute force Fourier transform (FT)" in the main text. Computing this 6–dimensional transform on the whole real space domain $(\mathbf{r}_1, \mathbf{r}_2)$ appears to require large resources. However, we observe:

- $\tilde{\omega}$ and $\tilde{\Phi}$ need to be calculated only once
- $\tilde{\Phi}(\mathbf{k}_1 + \mathbf{k}_2)$ is just $\tilde{\Phi}(\mathbf{k}_1)$ shifted by $\mathbf{k}_2$ in discrete Fourier transform language [4], and amplitudes with frequencies higher than $\frac{\pi}{\Delta}$ are neglected ($\Delta$ is the grid spacing in real space).
- For a given set of $\mathbf{r}_1$ and $\mathbf{k}_2$, the integrand of the $\mathbf{k}_2$–integral

  $$\int \sum_{\alpha\beta} \tilde{\Phi}_{\alpha\beta}(\mathbf{k}_1+\mathbf{k}_2)\tilde{\omega}_\alpha(-\mathbf{k}_1)\tilde{\omega}_\beta(-\mathbf{k}_2) e^{\mathrm{i}\mathbf{k}_1\cdot\mathbf{r}_1} d\,\mathbf{k}_1$$

  can be massively parallelized by CUDA [5, 6]. Furthermore, this expression does not depend on $\mathbf{r}_2$; thus, it needs to be evaluated only once for all $\mathbf{r}_2$.

For the actual computations, we use $2\times2\times2$ unit cells with a total of $128\times128\times128$ grid points. For the results of Fig. 1(b) in the main text, the brute force Fourier transform takes about 20 days (using one Nvidia TitanV graphics card).

Lattice symmetry demands that $\mathbf{k}_1+\mathbf{k}_2 = \mathbf{g}$ in Eq. (7) where $\mathbf{g}$ is a reciprocal lattice vector (RLV). This leads to the RLV expansion (Eq. (2) in the main text), where the RLV modes of the DCF are given by

$$\tilde{c}^{\rm cr}_{\mathbf{g}}(\mathbf{k}) = -\sum_{\alpha\beta} \tilde{\Phi}_{\alpha\beta}(\mathbf{g})\, \tilde{w}^{(\alpha)}\left(\gamma\mathbf{g}+\mathbf{k}\right) \tilde{w}^{(\beta)}\left(\gamma'\mathbf{g}-\mathbf{k}\right), \quad (8)$$

and $\gamma$ is an arbitray real constant. We employ a particular form of the corresponding RLV mode (with the choice $\gamma' = 1$ and $\gamma = 1-\gamma' = 0$ in Eq. (8) ):

$$\tilde{c}^{\rm cr}_{\mathbf{g}}(\mathbf{k}) = -\sum_{\alpha\beta} \tilde{\Phi}_{\alpha\beta}(\mathbf{g})\tilde{\omega}_\alpha(\mathbf{k})\tilde{\omega}_\beta(\mathbf{g}-\mathbf{k}) = -\sum_{\alpha\beta} \tilde{\Phi}_{\alpha\beta}(\mathbf{g})\tilde{\omega}_\alpha(\mathbf{k})\tilde{\omega}^*_\beta(\mathbf{k}-\mathbf{g}), \quad (9)$$

and thus the DCF through the RLV expansion is given by

$$c^{\rm cr}_{\rm RLV}(\mathbf{r}_1,\mathbf{r}_2) = -\frac{1}{(2\pi)^6}\sum_{\mathbf{g}} e^{\mathrm{i}\mathbf{g}\cdot\mathbf{r}_2}\int e^{-\mathrm{i}\mathbf{k}\cdot\mathbf{r}_2} \times \sum_{\alpha\beta} \tilde{\Phi}_{\alpha\beta}(\mathbf{g})\tilde{\omega}_\alpha(\mathbf{k})\tilde{\omega}^*_\beta(\mathbf{k}-\mathbf{g}) e^{\mathrm{i}\mathbf{k}\cdot\mathbf{r}_1} d\mathbf{k}. \quad (10)$$

In this form, the 6–dimensional integral of the brute force FT has been reduced to a 3–dimensional integral and a sum over RLV. The sum over RLV is organized in shells (these are RLV with the same modulus which are connected by lattice symmetry) which introduces some computational overhead. Here we observe that $\sum_{\alpha\beta} \tilde{\Phi}_{\alpha\beta}(\mathbf{g})\tilde{\omega}_\alpha(\mathbf{k})\tilde{\omega}^*_\beta(\mathbf{k}-\mathbf{g})e^{\mathrm{i}\mathbf{k}\cdot\mathbf{r}_1}$ is a 3–dimensional array of $\mathbf{k}$ and independent of $\mathbf{r}_2$; thus, one needs to evaluate it once for all $\mathbf{r}_2$.

For the results of Fig. 1(b) in the main text, the RLV sum up to $10^4$ shells takes about 4 days.

## III. NUMERICAL PROCEDURE FOR THE GENERALIZED ELASTIC CONSTANTS

Refs. [7, 8] introduce a density correlation matrix $J$:

$$\frac{1}{kT}J_{\mathbf{g}\mathbf{g}'}(\mathbf{q}) = \tilde{C}^{\rm id}_{\mathbf{g}-\mathbf{g}'} - \tilde{c}^{\rm cr}\left(\mathbf{g}+\mathbf{q}, -\mathbf{g}'-\mathbf{q}\right) \overset{\rm FMT}{=} \tilde{C}^{\rm id}_{\mathbf{g}-\mathbf{g}'} + \sum_{\alpha\beta} \tilde{\Phi}_{\alpha\beta}(\mathbf{g}-\mathbf{g}')\, \tilde{w}_\alpha(-\mathbf{g}-\mathbf{q})\tilde{w}_\beta(\mathbf{g}'+\mathbf{q}) \quad (11)$$

where $\mathbf{g}$ and $\mathbf{g}'$ are RLV's and $\mathbf{q}$ is a wave vector in the first Brillouin zone. Furthermore, $\tilde{C}^{\rm id}_{\mathbf{g}}$ is a RLV mode of the ideal gas part of the DCF. The generalized elastic constants are defined from the $\mathbf{q}\to 0$ limit of the following expression involving $J$:

$$\lambda_{\alpha\beta}(\mathbf{q}) = \sum_{\mathbf{g},\mathbf{g}'} g'_\alpha \tilde{\rho}^*_{\mathbf{g}'} J^*_{\mathbf{g},\mathbf{g}'}(\mathbf{q})\tilde{\rho}_{\mathbf{g}} g_\beta = \lambda_{\alpha\beta\gamma\delta}q_\alpha q_\beta + \mathcal{O}[\mathbf{q}^4],$$
$$\mu_\alpha(\mathbf{q}) = \sum_{\mathbf{g},\mathbf{g}'} \tilde{\rho}^*_{\mathbf{g}'} J^*_{\mathbf{g},\mathbf{g}'}(\mathbf{q})\tilde{\rho}_{\mathbf{g}} g_\beta = \mathrm{i}\mu_{\alpha\beta}q_\beta + \mathcal{O}[\mathbf{q}^2],$$
$$\nu(\mathbf{q}) = \sum_{\mathbf{g},\mathbf{g}'} \tilde{\rho}^*_{\mathbf{g}'} J^*_{\mathbf{g},\mathbf{g}'}(\mathbf{q})\tilde{\rho}_{\mathbf{g}} = \nu + \mathcal{O}[\mathbf{q}^2]. \quad (12)$$

Here, $\tilde{\rho}_{\mathbf{g}}$ are the RLV modes of the lattice–periodic density in the crystal. Since $C^{\rm id}(\mathbf{r}_1,\mathbf{r}_2) = \frac{\delta(\mathbf{r}_1-\mathbf{r}_2)}{\rho(\mathbf{r}_1)}$, the ideal gas part of the generalized elastic constants can be expressed in terms of the crystal density profile $\rho$ and its

derivative $\nabla\rho$; thus explicit calculation of $\tilde{C}^{\mathrm{id}}_{\mathbf{g}-\mathbf{g}'}$ is unnecessary. For the excess part, one observes that $\tilde{\Phi}_{\alpha\beta}(\mathbf{g}-\mathbf{g}')$ only needs to be computed once and $\omega(\mathbf{g}+\mathbf{q})$ is determined on the fly. We have again used graphics cards and CUDA. As an example, when determining

$$\nu(\mathbf{q}) = \sum_{\mathbf{g}}\sum_{\mathbf{g}'} \tilde{\rho}^*_{\mathbf{g}'} J^*_{\mathbf{g},\mathbf{g}'}(\mathbf{q})\tilde{\rho}_{\mathbf{g}} = \sum_{\mathbf{g}} \tilde{\rho}_{\mathbf{g}} \times \left(\sum_{\mathbf{g}'} J^*_{\mathbf{g},\mathbf{g}'}(\mathbf{q})\tilde{\rho}^*_{\mathbf{g}'}\right) \tag{13}$$

for a given $\mathbf{q}$, each thread is given one $\mathbf{g}$ and computes $\tilde{\rho}_{\mathbf{g}} \times \sum_{\mathbf{g}'} \tilde{\rho}^*_{\mathbf{g}'} J^*_{\mathbf{g},\mathbf{g}'}(\mathbf{q})$. The sum over all $\mathbf{g}$ is obtained by a sum over all threads. The generalized elastic constants are finally obtained by fitting $\lambda_{\alpha\beta}(\mathbf{q}), \mu_\alpha(\mathbf{q}), \nu(\mathbf{q})$ with the correct behavior for $\mathbf{q} \to 0$.

Computing $\lambda_{\alpha\beta}(\mathbf{q}), \mu_\alpha(\mathbf{q}), \nu(\mathbf{q})$ for a given $\mathbf{q}$ (with a RLV sum up to 1000 shells) takes about a few minutes GPU time (with one Nvidia TitanV graphics card).

We demonstrate the convergence of the RLV expansion for $\nu$ in Fig. 1. It shows that the sum is converged for an upper limit of shells above 100. In the main text, the first 1000 shells are used for the generalized elastic constants.

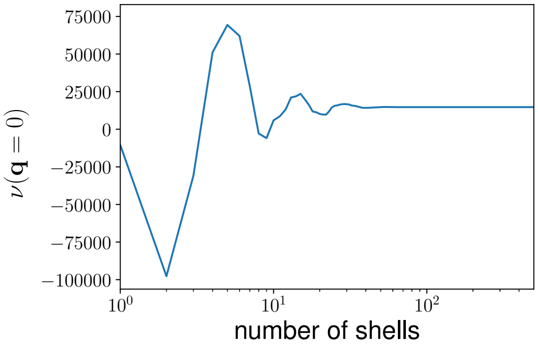


FIG. 1: $\nu(\mathbf{q}=0)$ versus number of shells at the melting point.

## IV. CONSISTENCY CHECK OF $\nu$

The generalized elastic constant $\nu$ describes the second–order response to a combination of "average density change–average density change" with no deformation of the lattice. Thus, it can be computed by scaling the crystal density profile by a factor $1+\delta$, i.e.

$$\begin{aligned}\frac{\mathcal{F}[(1+\delta)\times\rho]}{V} &= \frac{\mathcal{F}[\rho]}{V} + \delta\bar{\rho}\mu + \frac{\delta^2}{2V}\int d\mathbf{r}_1 \int d\mathbf{r}_2\, \rho(\mathbf{r}_1)\rho(\mathbf{r}_2)C(\mathbf{r}_1,\mathbf{r}_2) + \mathcal{O}(\delta^3) \\ &= \frac{\mathcal{F}[\rho]}{V} + \delta\bar{\rho}\mu + \frac{\delta^2}{2V}\nu + \mathcal{O}(\delta^3).\end{aligned} \tag{14}$$

Fitting $\frac{\mathcal{F}[(1+\delta)\times\rho]}{V}$ with a quadratic function in $\delta$, we obtain $\nu = 1.4705 \times 10^4$ at the melting point, which is consistent with $\nu$ determined from the density correlation matrix ($\nu = 1.4702 \times 10^4$).

## V. RELATION OF VOIGT ELASTIC CONSTANTS TO GENERALIZED ELASTIC CONSTANTS

The generalized elastic constants from the second order change in the DFT free energy (Eq. (7) in the main text) apply when strain and density can be varied independently. Coupling the coarse-grained density and strain via, $\delta\bar{\varrho} = -\bar{\varrho}u_{\alpha\alpha}$, the change of the microscopic density is caused by displacing particles, $\delta\varrho(\mathbf{r}) = -\nabla\cdot\big(\varrho(\mathbf{r})\mathbf{u}(\mathbf{r})\big)$, and is purely affine. This leads to the appearance of an elastic tensor $C^c_{\alpha\beta\gamma\delta}$ combining the generalized elastic constants from Eq. (7) of the main text after proper accounting for a Voigt-symmetric expression [8].

$$C^c_{\alpha\beta\gamma\delta} = \lambda_{\alpha\gamma\beta\delta} + \lambda_{\beta\gamma\alpha\delta} - \lambda_{\alpha\beta\gamma\delta} + \delta_{\alpha\beta}\mu_{\gamma\delta} + \mu_{\alpha\beta}\delta_{\gamma\delta} + \nu\delta_{\alpha\beta}\delta_{\gamma\delta}\ . \tag{15}$$

Defects may additionally contribute to $\delta\varrho(\mathbf{r})$ but the complete free energy functional of strain and defect concentration is still unknown from DFT. We interpret $C^c$ to apply at fixed defect density. Classical elasticity theory, used in Eq. (5) of the main text, only considers strain and includes density or volume changes into its trace [9], and thus its elastic constants should be considered to hold at fixed defect concentration as well. This is supported by a phenomenological approach [10], where a local thermodynamics containing strain and defect concentration was considered.

The remaining challenge then is to map $C^c$ to $C$ which proceeds by the following steps: Because of its origin in an expansion of the free energy functional, the constants $C^c_{\alpha\beta\gamma\delta}$ are second derivatives of the free energy per volume $f = F/V$ w.r.t symmetric strain. In contrast, in usual definitions like in [9] the elastic constants $C_{\alpha\beta\gamma\delta}$ are second derivatives of the free energy per particle $F/N$ w.r.t Lagrangian strain. Additionally, the expansion of $F/N$ for $C$ has to be formulated with the actual, strained volume, since the $F/V$ expansion for $C^c$ has no reference volume. To compare $C^c$ and $C$, these three differences (Lagrangian vs. symmetric strain, $F/V$ vs. $F/N$ and actual vs. reference volume) have to be considered. Then,

$$C_{\alpha\beta\gamma\delta} = C^c_{\alpha\beta\gamma\delta} - p\big(\delta_{\alpha\beta}\delta_{\gamma\delta} - \delta_{\alpha\gamma}\delta_{\beta\delta} - \delta_{\beta\gamma}\delta_{\alpha\delta}\big)\ , \tag{16}$$

which in an fcc crystal leads to the three Voigt elastic constants given in Eq. (9) of the main text. The above identification of $C^c$ as Birch coefficient [9] is consistent with the wave equation established in Ref. [7].

## VI. COMPUTING ELASTIC CONSTANTS USING AN EXPLICIT DEFORMATION OF THE FCC CRYSTAL

### A. Full minimization in deformed unit cells

Here we recapitulate the procedure to determine elastic constants by using explicit deformations [11]. Let $\mathbf{r}^i$ be the coordinate of particle $i$ in the undeformed system. Upon a homogeneous deformation, its coordinate is given by

$$\mathbf{r}_k^{\prime,i} = (u_{kl} + \delta_{kl})\mathbf{r}_l^i \tag{17}$$

with subscripts denoting Cartesian vector components, $u_{kl} = \partial_l u_k$ and $\mathbf{u}$ being the displacement field (here, the Einstein summation convention is used).

The elastic constants of a crystal are defined in terms of an expansion of the Helmholtz free energy $\mathcal{F}(N,V,T)$ in the Lagrangian strains $\eta_{ij}$, cf. Eq. (5) in the main text:

$$\frac{\mathcal{F}(\eta)}{V} = \frac{\mathcal{F}(0)}{V} - p\eta_{ij}\delta_{ij} + \frac{1}{2}C_{ijkl}\eta_{ij}\eta_{kl} + O(\eta^3) \tag{18}$$

with $p$ the pressure and $V$ the reference volume for the undeformed stat $\eta_{ij} = 0$. The FCC lattice has only 3 independent elastic constants ($C_{1111} \equiv C_{11}$, $C_{1122} \equiv C_{12}$ and $C_{1212} \equiv C_{44}$); thus we have

$$\begin{aligned}\frac{\mathcal{F}(\eta)}{V} = \frac{\mathcal{F}(0)}{V} &- p(\eta_{xx} + \eta_{yy} + \eta_{zz}) \\ &+ \frac{1}{2}C_{11}\left(\eta_{xx}^2 + \eta_{yy}^2 + \eta_{zz}^2\right) \\ &+ C_{12}\left(\eta_{xx}\eta_{yy} + \eta_{xx}\eta_{zz} + \eta_{yy}\eta_{zz}\right) \\ &+ 2C_{44}\left(\eta_{xy}\eta_{xy} + \eta_{xz}\eta_{xz} + \eta_{yz}\eta_{yz}\right) + \mathcal{O}(\eta^3)\end{aligned} \tag{19}$$

and the $\eta$ tensor is related to $u_{kl}$ through

$$\eta_{kl} = \frac{1}{2}(u_{kl} + u_{lk} + u_{mk}u_{ml}). \tag{20}$$

Therefore, we choose 3 types of deformation to determine the elastic constants.

1. **Isotropic:** $u_{xx} = u_{yy} = u_{zz} = \delta$ ($\eta_{xx} = \eta_{yy} = \eta_{zz} = \delta + \frac{\delta^2}{2}$) and 0 otherwise, and

$$\frac{\mathcal{F}(\delta)}{V} = \frac{\mathcal{F}(0)}{V} - 3p\delta + \left(-\frac{3}{2}p + \frac{3}{2}C_{11} + 3C_{12}\right)\delta^2 + \mathcal{O}(\delta^3). \tag{21}$$

2. **Uniaxial:** $u_{xx} = \delta$ ($\eta_{xx} = \delta + \frac{\delta^2}{2}$) and 0 otherwise, and

$$\frac{\mathcal{F}(\delta)}{V} = \frac{\mathcal{F}(0)}{V} - p\delta + \left(-\frac{1}{2}p + \frac{1}{2}C_{11}\right)\delta^2 + \mathcal{O}(\delta^3). \tag{22}$$

3. **Shear:** $u_{xy} = \delta$ ($\eta_{xy} = \eta_{yx} = \frac{\delta}{2}, \eta_{yy} = \frac{\delta^2}{2}$) and 0 otherwise, and

$$\frac{\mathcal{F}(\delta)}{V} = \frac{\mathcal{F}(0)}{V} + \left(-\frac{1}{2}p + \frac{1}{2}C_{44}\right)\delta^2 + \mathcal{O}(\delta^3). \tag{23}$$

We also have used biaxial deformation, $u_{xx} = u_{yy} = \delta$ (and 0 otherwise), to check $C_{11}$ and $C_{12}$.

The free energy of the deformed states is determined by a full minimization of the FMT functional (no parameterizations of the density profile as e.g. in Ref. [11]). This requires the use of numerical boxes of cuboid shape with periodic boundary conditions. It is worth to note that the deformations of first and second type can be done with only one (conventional) unit cell. However, due to the periodic boundary conditions, the third type needs a long numerical box for small deformations. For example, a lattice particle at coordinate $(l_x, l_y, z)$ in the undeformed state will be at $(l_x + l_y \times \delta, l_y, z)$ upon the shear deformation chosen above. With the periodic boundary condition for the density profile ($\rho(l_x, l_y, z) = \rho(0, l_y, z)$), $l_y \times \delta$ must be $n \times l_x$ with $n = \pm1, \pm2, \pm3....$ We illustrate this in Fig. 2. As a consequence, for $\delta = 0.01$, we need at least 100 unit cells. For the results in the main text,

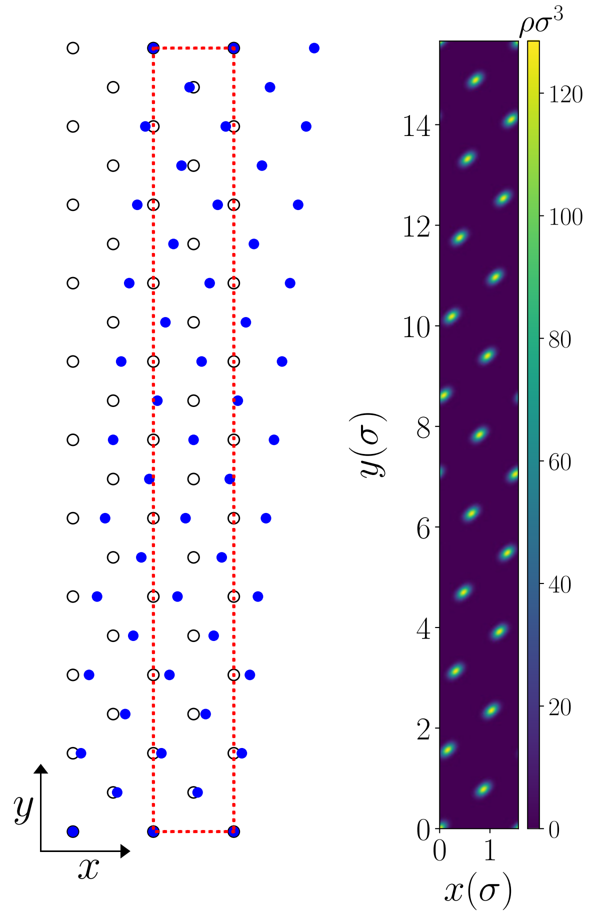


FIG. 2: $\rho(x, y, 0)$ at the melting point under $u_{xy} = 0.1$ and 0 otherwise. (a) Schematic plot. Black circles are lattice sites in the undeformed state and blue dots lattice sites in the sheared state. The rectangular box of red dashed lines is one periodic box of the deformed lattice (blue dots). (b) equilibrium $\rho(x, y, 0)$ under shear.

$C_{44}$ is determined using $\delta = 0, \pm\frac{1}{50}, \pm\frac{1}{75}$ and $\pm\frac{1}{100}$. In contrast, $C_{11}$ and $C_{12}$ are determined with much smaller $\delta$'s in the range of $[-10^{-5}, 10^{-5}]$.

### B. Affine change of density and consistency check with elastic constants from the DCF route

The density distribution in a deformed unit cell can be approximated by an "affine stretch" and a global rescaling to keep constant the number of particles in the unit cell:

$$\rho'(\mathbf{r}+\mathbf{u}) = \rho(\mathbf{r}) \times \left(1 + \frac{\delta\bar{\rho}}{\bar{\rho}}\right) . \tag{24}$$

Eq. (6) in the main text then is the density change to first order in $\mathbf{u}$ and $\delta\bar{\rho}$ of such an affinely stretched density:

$$\begin{aligned}\delta\rho(\mathbf{r}) &= \rho(\mathbf{r}-\mathbf{u})\left(1+\frac{\delta\bar{\rho}}{\bar{\rho}}\right) - \rho(\mathbf{r}) \\ &\approx -\mathbf{u}(\mathbf{r})\cdot\nabla\rho(\mathbf{r}) + \rho(\mathbf{r})\frac{\delta\bar{\rho}(\mathbf{r})}{\bar{\rho}} .\end{aligned} \tag{25}$$

However, one must realize that $\rho'$ is not the density in an equilibrated deformed unit cell, and thus the free energy and elastic constants are larger than obtained from density distributions after full minimization. In Tab. I, the elastic constants from DCF route (Eq. (9) in the main text), and from non–equilibrium and equilibrium density distributions are shown. The elastic constants from the first two routes agree very well, while they differ from the equilibrium ones. On the one hand, this confirms the numerical results from the DCF route via an independent route. On the other hand, this implies that the "affine stretch" approximation (Eq. (6) in the main text) requires modification for a full quantitative determination of all elastic constants; this is currently under investigation.

| | DCF | non–eq–FMT | eq–FMT |
|---|---|---|---|
| $C_{11}$ | 124.7 | 123.2 | $79.7 \pm 0.3$ |
| $C_{12}$ | 61.58 | 60.96 | $17.8 \pm 0.3$ |
| $C_{44}$ | 58.81 | 59.0 | $49.5 \pm 0.5$ |

TABLE I: Elastic constants by DCF, affine stretch approximation (non–eq–FMT) and equilibrium $\rho$ (eq–FMT) at the melting point ($\eta = 0.545$ with $n_{\text{vac}} = 2.18 \times 10^{-5}$).


[1] R. Roth, J. Phys. Condens. Matter **22**, 063102 (2010).

[2] T. Bernet, E. Müller, and G. Jackson, J. Chem. Phys. **152**, 224701 (2020).

[3] M. Mortazavifar, *Equilibrium properties of crystals in the hard–sphere and the Asakura–Oosawa Model* , Ph.D. thesis, Eberhard Karls Universität Tübingen (2016), `https://publikationen.uni-tuebingen.de/xmlui/handle/10900/74611`.

[4] M. Frigo and S. G. Johnson, ASCL , 1201 (2012).

[5] J. Nickolls, I. Buck, M. Garland, and K. Skadron, Queue **6**, 40 (2008).

[6] D. Stopper and R. Roth, J. Chem. Phys **147**, 064508 (2017).

[7] C. Walz and M. Fuchs, Phys. Rev. B **81**, 134110 (2010).

[8] J. M. Häring, C. Walz, G. Szamel, and M. Fuchs, Phys. Rev. B **92**, 184103 (2015).

[9] D. C. Wallace, in *Solid state physics*, Vol. 25 (Elsevier, 1970) pp. 301–404.

[10] P. Fleming and C. Cohen, Phys. Rev. B **13**, 500 (1976).

[11] B. B. Laird, J. Chem. Phys **97**, 2699 (1992).
